# Supplementary material for: TriviaQA: A Large Scale Distantly Supervised Challenge Dataset for Reading Comprehension
Source: arXiv:1705.03551 source file (2017-05-13)
Supplement: Supplementary file 1 [file appendix.tex]

\appendix

\section{Features for the entity classifier}
\label{sec:supplemental}

We describe three different types of features we developed: entity features, type features, and context features. We use the running example, \emph{Which politician won the Nobel Peace Prize in 2009?} with the answer \emph{Barack Obama} to explain the features.

\begin{enumerate}[wide, labelwidth=!, labelindent=0pt]
\item \emph{Entity features}: These features are designed to discourage candidates that a) appear in the question, and b) contain a subset of words from the ground truth. For example, we aim to discourage entities in the question such as \emph{Nobel Peace Prize} and sub-spans like \emph{Barack}. %are occur in the question or are lexical variations of question words.
\begin{itemize}
 \item Proportion of entity words occurring in the question $q$. %($\frac{| w \in e \wedge q |}{| w \in e |}$) 
\item Average cosine similarity of entity word embeddings with the embedding of the closest (by cosine similarity) question word.\footnote{We use the 100-dimensional pre-trained GloVe word embeddings \cite{pennington2014glove}.}

\item Binary feature indicating whether another candidate entity contains a subset of words from the entity $e$.

\item Binary feature indicating whether all tokens in the entity $e$ are stop words.

% $\sum_i \max_w cos(e[i], w) \forall w \in q) / |e|$
\end{itemize}

\item \emph{Type features}: These features encourage the selection of entities that match possible answer type hints mentioned in the question. For our running example, we expect these features to prefer entities of the type {\tt politician} over other entities. Type features assume an external knowledge base which lists types for each entity.\footnote{We use the Wikipedia type ontology.}
\begin{itemize}
% \item Highest match over every question n-gram and every category of $e$ ($n \in [1,5]$).

\item Aggregation of embedding based similarities between question n-grams and category n-grams of $e$. We use $\sum$ and $\max$ as aggregation functions.

%$\max_c (\sum_i ngrams(c)[i] \in question ) / |ngrams(c)|) c \in cats(e)$

\end{itemize}

% \item \emph{IR features}: These features prefer entities that occur frequently and in top ranked pages. 
% \begin{itemize}
% \item The proportion of search documents and snippets $D$ (if available)  for question $q$ in the top-$k$ results that contain the entity $e$ ($k \in \{1, 5, 10\}$)

% \item The total number of evidence documents and snippets $D$ for question $q$ with the entity $e$ 
% \end{itemize}

\item \emph{Context features}: These features match the context around the entity $e$ with the question. For example, assuming that the evidence is of high quality, we expect the context around \emph{Barack Obama} to match question phrases like \emph{Nobel Peace Prize} and \emph{2009}.
\begin{itemize}
\item Aggregation of embedding based similarities between question n-grams and context n-grams of $e$. We use $\sum$ and $\max$ as aggregation functions.
\end{itemize}
\end{enumerate}
